# Supplementary material for: 2D Points Curve Reconstruction Survey and Benchmark
Source: arXiv:2103.09583 source file (2021-03-17)
Supplement: Supplementary file 1 [file appendix.tex]

\appendix
\section{Gauss-Newton for Dummies}

\begin{algorithm}
\caption{Gauss-Newton}
\label{gaussnewton}
\begin{algorithmic}[1]

\Procedure{Step}{$\sphere_{t-1}$}

%\State $J \gets \text{zeros}(\text{n_constraints}, d)$
%\State $R \gets \text{zeros}(\text{n_constraints})$

\EndProcedure

\end{algorithmic}
\end{algorithm}

\section{Gradients of Energy Components}
Gradients are written in the form $\nabla_\sphere f(\sphere) = \left[\nabla_\c f(\sphere), \frac{\partial f(\sphere)}{\partial \r} \right]$.

\paragraph{Inscription Term}
Given oriented surface point $(\point_n, \normal_n)$:
\begin{equation}
\nabla_\sphere \kernel_n(\bar\c_n) = [, 0]
\end{equation}
\begin{equation}
\nabla_\sphere \sdf_\text{plane}(\sphere) = [\normal_n, -1]
\end{equation}
\begin{equation}
\nabla_\sphere \sdf_\text{point}(\sphere) = \left[\frac{\c - \point_n}{\|\c - \point_n\|_2}, -1 \right]
\end{equation}
\paragraph{Maximality Term}
We include the $\ell^1$ maximality term in our least-squares system with residual and gradient:
\begin{equation}
\mathbf{R}_\text{maximal} = \sqrt{\r_\text{max} - \r}
\end{equation}
\begin{equation}
\nabla_\sphere \mathbf{R}_\text{maximal} = \left[0, -\frac{1}{2}(\r_\text{max} - \r)^{-\frac{1}{2}} \right]
\end{equation}
\paragraph{Pinning Term}
Given pinning cone $\mathcal{C}$ of aperature $\pinangle$ defined by surface point $(\point_n, \normal_n)$:
\begin{equation}
d = 
\sdf_\mathcal{C}(\c) = \| \c - \point_n - \normal_n d \|_2 - d \sin(\pinangle)
\end{equation}
\begin{equation}
\nabla_\sphere \sdf_\mathcal{C}(\c) = [, 0]
\end{equation}
